# Supplementary material for: Composing Networks of Automated Market Makers
Source: arXiv:2106.00083 source file (2021-08-31)
Supplement: Supplementary file 1 [file appendix.tex]

Material we may or may not want to include

\begin{lemma}
  An $n$-dimensional AMM $A$ can be written uniquely as the image of a strictly convex, continuous function in $n$ coordinates.
\end{lemma}

\begin{proof}
    Consider some $\by$ on the manifold $A(\by) = 0$.
    Without loss of generality fix the first $n$ coordinates of $\by$.
    Define
    $f(y_0,\ldots,y_{n-1}) = \set{z \in \PosReals : A(y_0,\ldots,y_{n-1},z)=0}$.
    Note $y_n \in f(y_0,\ldots,y_{n-1})$ so 
    $|f(y_0,\ldots,y_{n-1})| \neq \emptyset$.
    Suppose there are two distinct elements $z,z^{'} \in f(y_0,\ldots,y_{n-1}) $
    where $z < z^{'}$.
    Since $A(y_0,\ldots,y_{n-1},z^{'}) = 0$ we know by Lemma 12,
    it is a stable point for some $\bv \in \int(\Delta^n)$.
    But $\bv \cdot (y_0,\ldots,y_{n-1},\bz) < \bv \cdot (y_0,\ldots,y_{n-1},z^{'})$ by construction,
    a contradiction because $(y_0,\ldots,y_{n-1})$ is a stable point for $\bv$.
    Hence $f(y_0,\ldots,y_{n-1})$ is a function.
    Because $\upper(A)$ is a strictly convex set,
    $f$ is a strictly convex function.
    Convex functions on Euclidean spaces are continuous, 
    so $f$ is continuous.
\end{proof}
